# Supplementary material for: PokeGym: Mastering Long-Horizon, Open-World 3D Games via Graph-Guided Multimodal Evolution
Source: arXiv:2604.08340 source file (2026-11-30)
Supplement: Supplementary file 1 [file supp-peramble.tex]

% \def\eg{\emph{e.g.~}} \def\Eg{\emph{E.g.~}}
% \def\ie{\emph{i.e.~}} \def\Ie{\emph{I.e.~}}
% \def\cf{\emph{cf.~}} \def\Cf{\emph{Cf.~}}
% \def\etc{\emph{etc.~}} \def\vs{\emph{vs.~}}
% \def\wrt{w.r.t.~} \def\dof{d.o.f.~}
% \def\iid{i.i.d.~} \def\wolog{w.l.o.g.~}
% \def\etal{\emph{et al.~}}
% 
% \usepackage[T1]{fontenc}
% \usepackage{amssymb}   % 提供对勾符号 \checkmark
% % \usepackage{textcomp}   % 提供直引号 \textquotedbl
% 
% \usepackage{graphicx}
% \usepackage{tabularx}  % 自动调整列宽
% \usepackage{makecell}  % 支持表头换行
% \usepackage{multirow}   % 处理多行合并
% \usepackage{graphicx}   % 用于调整表格宽度 \resizebox
% \usepackage{colortbl} % 用于表格行/列染色
% \usepackage{xcolor}
% %\usepackage[table]{xcolor}   % 提供 \rowcolor 等表格颜色命令
% %\usepackage{orcidlink}
% \usepackage{amsmath}
% %\usepackage{cleveref}
% \usepackage{url}
% \usepackage{enumitem}
% \usepackage{algorithm}
% \usepackage{algpseudocode}
% \usepackage{booktabs}
% \usepackage{tcolorbox}
% \tcbuselibrary{breakable}  % 允许 promptbox 跨页
% \usepackage{caption}    % 让 strip 内也能用 \caption
% %\usepackage{cuted}      % 提供 strip 环境
% \usepackage{etoolbox}     % 用于全局环境钩子
% \usepackage{listings}
% 
% 
% \definecolor{za-pink}{rgb}{0.79, 0.62, 0.70}
% \definecolor{za-grey}{rgb}{0.43, 0.45, 0.48}
% \definecolor{za-dark}{rgb}{0.19, 0.16, 0.12}
% \definecolor{za-green}{rgb}{0.25, 0.71, 0.48}
% 
% %\newcommand{\pokeza}{\textbf{\textcolor{za-pink}{Pokémon} \textcolor{za-grey}{Legends}:~\textcolor{za-dark}{Z}-\textcolor{za-green}{A}}}
% 
% \newcommand{\pokeza}{\textbf{\textcolor{black}{Pokémon} \textcolor{black}{Legends}:~\textcolor{black}{Z}-\textcolor{black}{A}}}
% 
% \newcommand{\no}{$\times$}
% \newcommand{\yes}{\checkmark}
% 
% 
% 
% 
% 
% % 自定义一个叫 promptbox 的环境
% \newtcolorbox{promptbox}[1][]{
% 	colback=yellow!15!white,   % 背景色：更饱和的浅黄色
% 	colframe=yellow!90!black, % 边框色：更亮的黄色
% 	fonttitle=\bfseries,    % 标题字体加粗
% 	title=#1,               % 允许传入标题
% 	boxrule=0.5mm,          % 边框粗细
% 	arc=2mm,                % 圆角弧度
% 	before upper={\setlength{\parskip}{0pt}\setlength{\parindent}{0pt}\small},
% 	left=2mm, right=2mm, top=2mm, bottom=2mm % 内边距
% }
% % 定义高亮颜色
% \definecolor{highlightgray}{gray}{0.9}
% 
% 
% 
% %\usepackage{marvosym}
% %\newcommand{\corresponding}{\texorpdfstring{$^{\textrm{\Letter}}$}{}}
% %\usepackage{cuted} 
% 
% %\newlength{\IEEEteaserwidth}
% %\setlength{\IEEEteaserwidth}{\dimexpr2\columnwidth+\columnsep\relax}
\def\eg{\emph{e.g.~}} \def\Eg{\emph{E.g.~}}
\def\ie{\emph{i.e.~}} \def\Ie{\emph{I.e.~}}
\def\cf{\emph{cf.~}} \def\Cf{\emph{Cf.~}}
\def\etc{\emph{etc.~}} \def\vs{\emph{vs.~}}
\def\wrt{w.r.t.~} \def\dof{d.o.f.~}
\def\iid{i.i.d.~} \def\wolog{w.l.o.g.~}
\def\etal{\emph{et al.~}}

\usepackage[T1]{fontenc}
\usepackage{amssymb}   % 提供对勾符号 \checkmark
% \usepackage{textcomp}   % 提供直引号 \textquotedbl

\usepackage{graphicx}
\usepackage{tabularx}  % 自动调整列宽
\usepackage{makecell}  % 支持表头换行
\usepackage{multirow}   % 处理多行合并
\usepackage{graphicx}   % 用于调整表格宽度 \resizebox
\usepackage{colortbl} % 用于表格行/列染色
\usepackage{xcolor}
%\usepackage[table]{xcolor}   % 提供 \rowcolor 等表格颜色命令
%\usepackage{orcidlink}
\usepackage{amsmath}
%\usepackage{cleveref}
\usepackage{url}
\usepackage{enumitem}
\usepackage{algorithm}
\usepackage{algpseudocode}
\usepackage{booktabs}
\usepackage{tcolorbox}
\tcbuselibrary{breakable}  % 允许 promptbox 跨页
\usepackage{caption}    % 让 strip 内也能用 \caption
%\usepackage{cuted}      % 提供 strip 环境
\usepackage{etoolbox}     % 用于全局环境钩子
\usepackage{listings}


\definecolor{za-pink}{rgb}{0.79, 0.62, 0.70}
\definecolor{za-grey}{rgb}{0.43, 0.45, 0.48}
\definecolor{za-dark}{rgb}{0.19, 0.16, 0.12}
\definecolor{za-green}{rgb}{0.25, 0.71, 0.48}

%\newcommand{\pokeza}{\textbf{\textcolor{za-pink}{Pokémon} \textcolor{za-grey}{Legends}:~\textcolor{za-dark}{Z}-\textcolor{za-green}{A}}}

\newcommand{\pokeza}{\textbf{\textcolor{black}{Pokémon} \textcolor{black}{Legends}:~\textcolor{black}{Z}-\textcolor{black}{A}}}

\newcommand{\no}{$\times$}
\newcommand{\yes}{\checkmark}





% 自定义一个叫 promptbox 的环境
\newtcolorbox{promptbox}[1][]{
colback=black!2,
colframe=black!35,
colbacktitle=black!7,
coltitle=black,
fonttitle=\normalfont\small\bfseries,
fontupper=\normalfont\small,
title=#1,
boxrule=0.4pt,
arc=1mm,
% before upper={\raggedright\setlength{\parindent}{0pt}\setlength{\parskip}{2pt}},
before upper={\setlength{\parindent}{0pt}\setlength{\parskip}{0pt}}, 
left=2mm, right=2mm, top=2mm, bottom=2mm
}
% 定义高亮颜色
\definecolor{highlightgray}{gray}{0.9}



%\usepackage{marvosym}
%\newcommand{\corresponding}{\texorpdfstring{$^{\textrm{\Letter}}$}{}}
%\usepackage{cuted} 

%\newlength{\IEEEteaserwidth}
%\setlength{\IEEEteaserwidth}{\dimexpr2\columnwidth+\columnsep\relax}
